# Supplementary material for: Electrically and optically active charge carrier traps in silicon-doped few-layer GaSe
Source: arXiv:2602.03964 ancillary file (2026-02-03)
Supplement: Supplementary file 1 [file Supplementary_Information.pdf]

## Supplementary Information

### Electrically and optically active charge carrier traps in silicon-doped few-layer GaSe

*M. Bissolo,<sup>1,\*</sup> R. Li,<sup>1,2</sup> M. Ogura,<sup>3</sup> Z. Sofer,<sup>4</sup> S. Polesya,<sup>3</sup> D. Han,<sup>5</sup> A. W. Holleitner,<sup>1</sup> C. Kastl,<sup>1</sup> G. Koblmüller,<sup>1,6</sup> H. Ebert,<sup>3</sup> E. Zallo,<sup>1,†</sup> and J. J. Finley<sup>1</sup>*

*1)Walter-Schottky-Institut and TUM School of Natural Sciences, Technische Universität München, Am Coulombwall 4,85748 Garching, Germany*

*2)Current address: Max Planck Institute for Chemical Physics of Solids, Nöthnitzer Str. 40, 01187 Dresden, Germany*

*3)Department of Chemistry, Ludwig-Maximilians-Universität München, Butenandtstrasse 5-13, 81377 München, Germany*

*4)Department of Inorganic Chemistry, University of Chemistry and Technology Prague, Technická 5, 16628 Prague, Czech Republic*

*5)School of Materials Science and Engineering, Jilin University, Changchun, 130012 China*

*6)Institute of Physics and Astronomy, Technical University Berlin, Hardenbergstrasse 36, 10623 Berlin, Germany*

*Germany*

*\*E-mail: [michele.bissolo@tum.de](mailto:michele.bissolo@tum.de)*

*†E-mail: [eugenio.zallo@tum.de](mailto:eugenio.zallo@tum.de)*

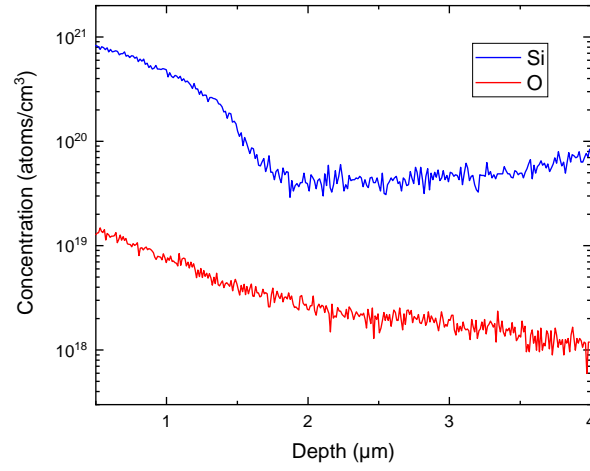

**Figure S 1:** Si and O impurity concentration as a function of depth as extracted from SIMS.

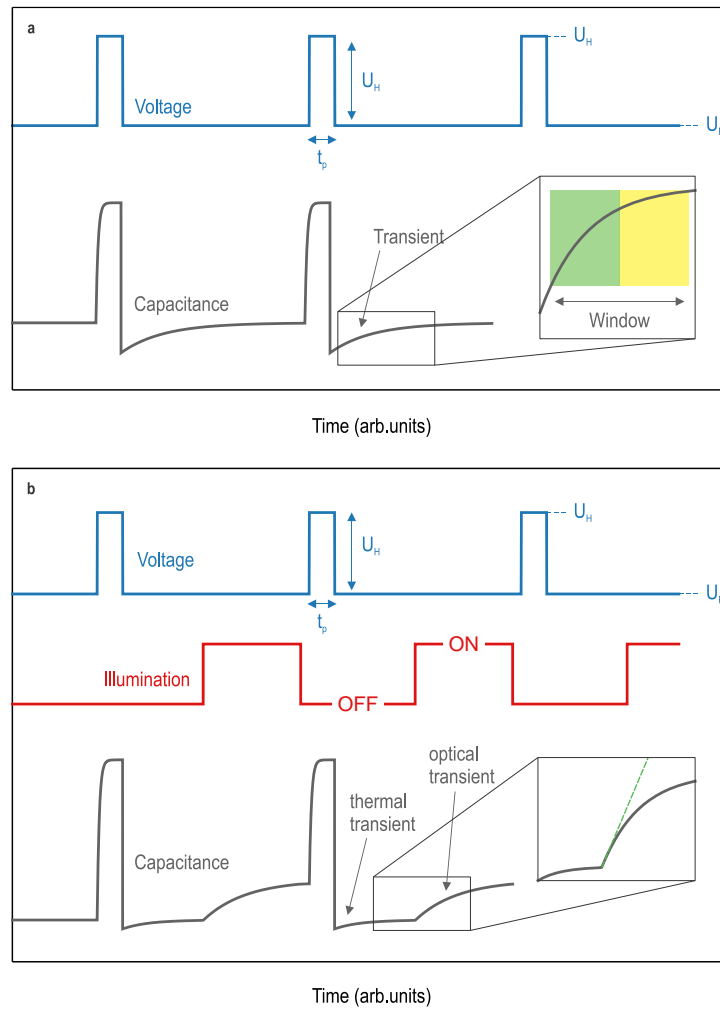

**Figure S 2:** Pulse sequences for DLTS (a) and DLOS (b).

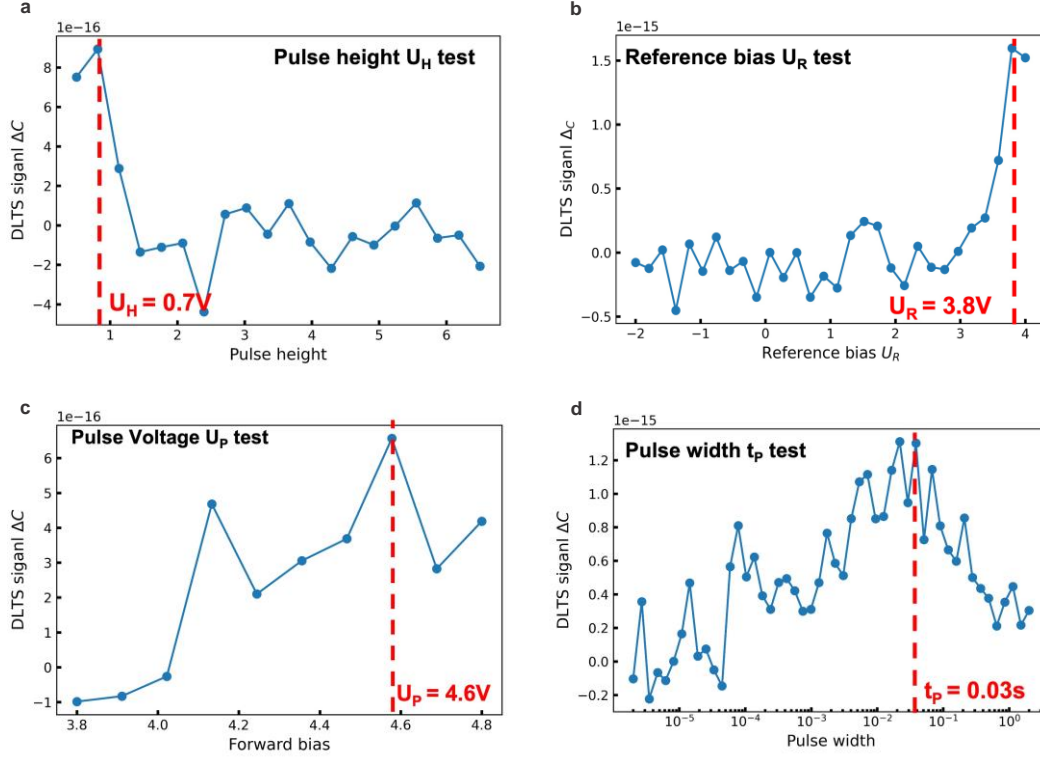

**Figure S 3:** (a)-(d) Parameter optimization for pulse height  $U_H$ , reference bias  $U_R$ , pulse voltage  $U_P$  and pulse width  $t_p$  with the condition: (a) fixed  $U_P$  at 4.5 V, varying  $U_H$  from -2 V to 4 V. (b) fixed  $U_H$  at 0.7 V, varying  $U_R$  from -2 V to 4 V. (c) fixed  $U_R$  at 3.8 V, varying  $U_H$  from 0 V to 1 V. (d) fixed  $U_R=3.7$  V,  $U_P=4.6$  V, varying  $t_p$  from 1  $\mu$ s to 3 s. The vertical red dashed lines indicate the optimized parameters for  $U_H$ ,  $U_R$ ,  $U_P$ , and  $t_p$  (0.7 V, 3.8 V, 4.6 V, and 0.03 s, respectively).

#### Note S1: Principles of Deep Level Transient Spectroscopy (DLTS):

DLTS is based on the measurement of capacitance transients arising from carrier emission from defects. The transients are obtained by first filling the traps with a voltage pulse. After the pulse, the defects emit carriers thermally with an exponential decay  $C_0 - C(t) = \Delta C \cdot e^{-e_n t} = \Delta C \cdot e^{-t/\tau}$ , where the emission rate  $e_n = 1/\tau$  depends on temperature as  $e_n = \sigma_n v_{th} N_C e^{-(E_C - E_T)/kT}$ .

For 2D materials, the thermal velocity  $v_{th}^{(2D)}$  and the effective density of states  $N_C^{(2D)}$  are given by  $v_{th}^{(2D)} = \sqrt{\frac{2kT}{m^*}}$ ,  $N_C^{(2D)} = \frac{8\pi m^* kT}{h^2}$ . Substituting these into the equation describing the emission rate) yields the 2D Arrhenius relation:  $\ln(\tau T^{3/2}) = \frac{E_C - E_T}{kT} - \ln(K_{2D} \sigma_n)$ , where  $K_{2D} = v_{th} N_C$ .

The defect energy levels and capture cross sections are extracted from the temperature dependence of the emission rate. Because transients can involve multiple traps, the DLTS signal is obtained using a correlation (weighting) technique rather than direct fitting of the capacitance

decay. In this work, we use a rectangular Lock-in weighting function to improve the signal-to-noise ratio. The emission rate for each trap is determined from the DLTS signal maximum, which occurs when the rate time window matches the trap lifetime. The choice of time window strongly affects the peak shape and sensitivity; here, a fixed ratio  $t_2/t_1=1.048$  is used. With the temperature-dependent emission rates, trap energies and capture cross sections are obtained from the Arrhenius relation.

### Note S2: Principles of Deep level Optical Spectroscopy (DLOS):

In DLOS, the measurement is performed at cryogenic temperatures, so that defects have very long lifetimes compared to the measurement timescale, such that the thermal emission is negligible for most traps. The pulse sequence is as follows:

1. Defects are first populated with a voltage pulse, filling the available trap states.
2. Very fast thermal transients occur immediately for traps very close to the band edge, which are effectively ignored in subsequent steps.
3. The sample is then illuminated with a light pulse of a specific wavelength, which excites carriers out of the traps, causing a change in capacitance.

The change in capacitance can be expressed as  $C \approx C_0 \left(1 - \frac{n_T(t)}{2N_D}\right)$ . Here  $N_D$  is the doping density,  $n_T$  the density of occupied defects. At  $t=0$ , all defects are occupied, such that only transitions to the bands are possible and  $\frac{dn_T}{dt} = -e_{optical} \cdot n_T$  is valid. By fitting the slope of the capacitance immediately after illumination the optical emission rate  $e_{optical}$  can be extracted:  $\left(\frac{dC}{dt}\right)_0 \propto -e_{optical} \cdot N_T = \sigma_n \Phi N_T$ , where  $\Phi$  is the photon flux and  $\sigma_n$  the optical capture cross section.

This procedure is repeated for many wavelengths. By plotting the optical emission rate as a function of photon energy, the trap photoionization thresholds are obtained.

### Note S3: Principles of Thermal Admittance Spectroscopy (TAS):

TAS probes defect energy levels and capture cross sections by monitoring the frequency-dependent capacitance response of defects close to the band edges, which can thus be filled and emptied at frequencies higher than a few tens of hertz.

For a specific trap, there exists a demarcation frequency  $\omega_0$ : for  $\omega < \omega_0$ , traps can respond to the AC voltage and contribute to the capacitance; for  $\omega > \omega_0$ , they cannot.

The demarcation frequency is extracted from the differential capacitance spectrum measured across temperatures. The trap energy  $E_T$  and capture cross section  $\sigma_n$  are obtained from the temperature dependence of the emission rate  $1/t_e = \omega_0$  using the thermionic emission relation explained in Note S1.

**Note S4: Voltage-chemical potential relation in 2D materials:**

In 2D materials, the applied voltage is related to the chemical potential through the series combination of the geometric capacitance  $C_{\text{geom}}$  and the quantum capacitance  $C_Q$ :

$$V(\mu) = \frac{\mu - \mu_0}{e} + \frac{Q(\mu)}{C_{\text{geom}}}.$$

At low temperatures, the charge is given by  $Q(\mu) = \int_{-\infty}^{\mu} \text{DOS}(E) dE$ .

Assuming an exponential band-tail density of states  $\text{DOS}(E) = D_0 \exp\left(\frac{E}{E_0}\right)$ , the voltage–chemical potential relation becomes

$$V(\mu) = \frac{\mu - \mu_0}{e} + \frac{eD_0E_0}{C_{\text{geom}}} \exp\left(\frac{\mu}{E_0}\right),$$

directly linking the applied voltage to the chemical potential and band-tail parameters.

## Formation energy of intrinsic defects in GaSe

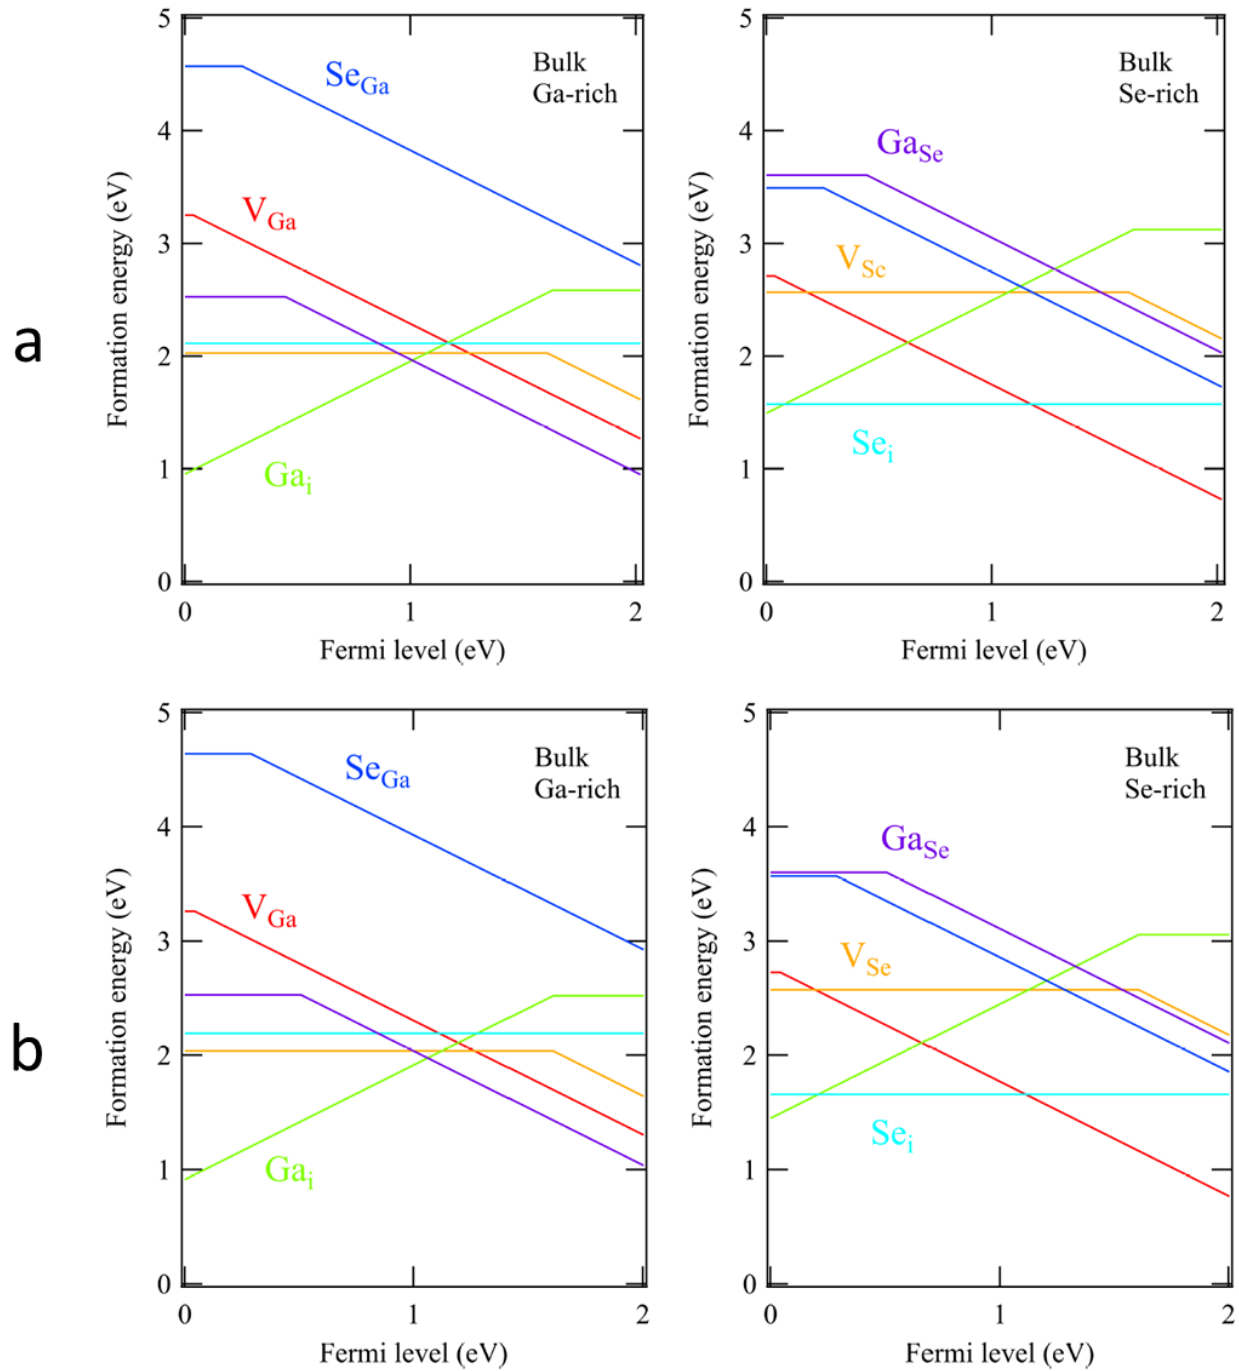

**Figure S 4:** Formation energy of defects in GaSe for Ga-rich (left) and Se-rich (right) conditions in bulk (a)  $\epsilon$ -GaSe and (b)  $\beta$ -GaSe. In the Ga-rich case, metallic Ga is assumed as reservoir and, in the Se-rich case,  $\text{Ga}_2\text{Se}_3$  is assumed.

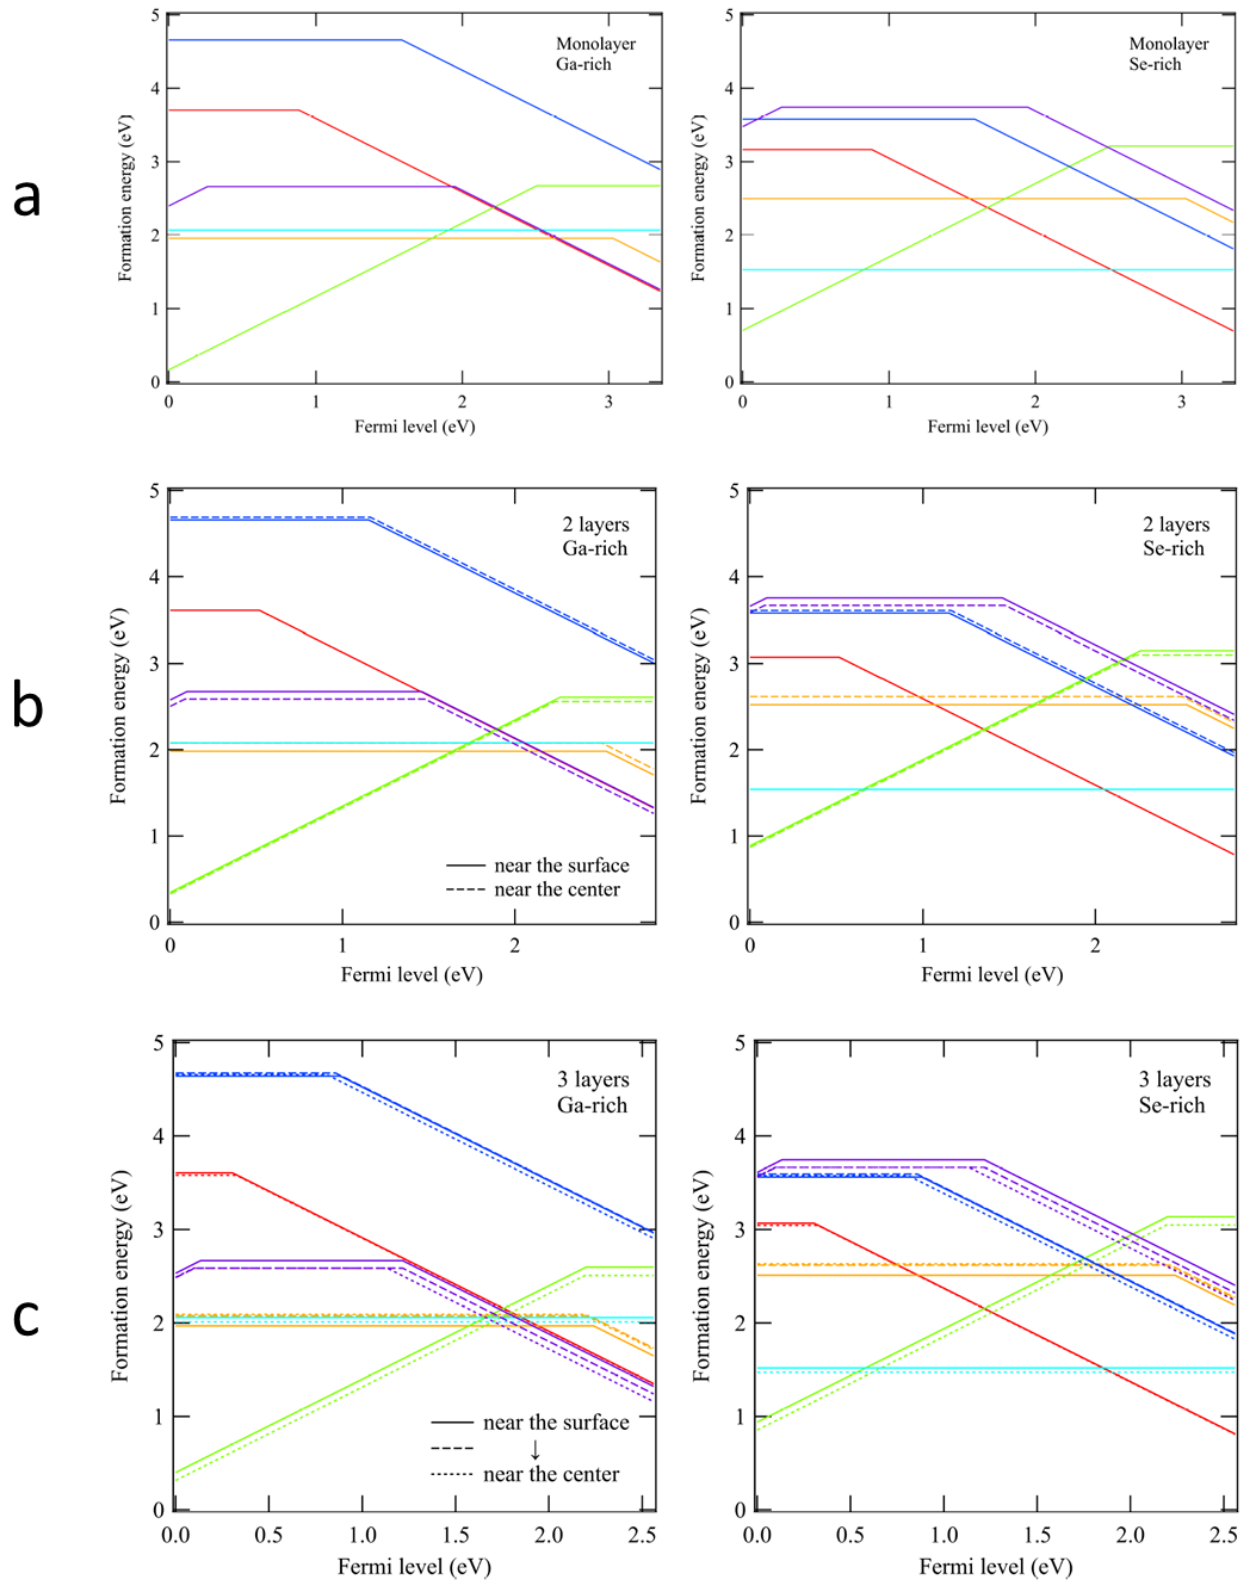

**Figure S 5:** Formation energy of defects in GaSe for Ga-rich (left) and Se-rich (right) conditions in (a) monolayer, (b) bilayer and (c) trilayer GaSe. In the Ga-rich case, metallic Ga is assumed as reservoir and, in the Se-rich case,  $\text{Ga}_2\text{Se}_3$  is assumed.

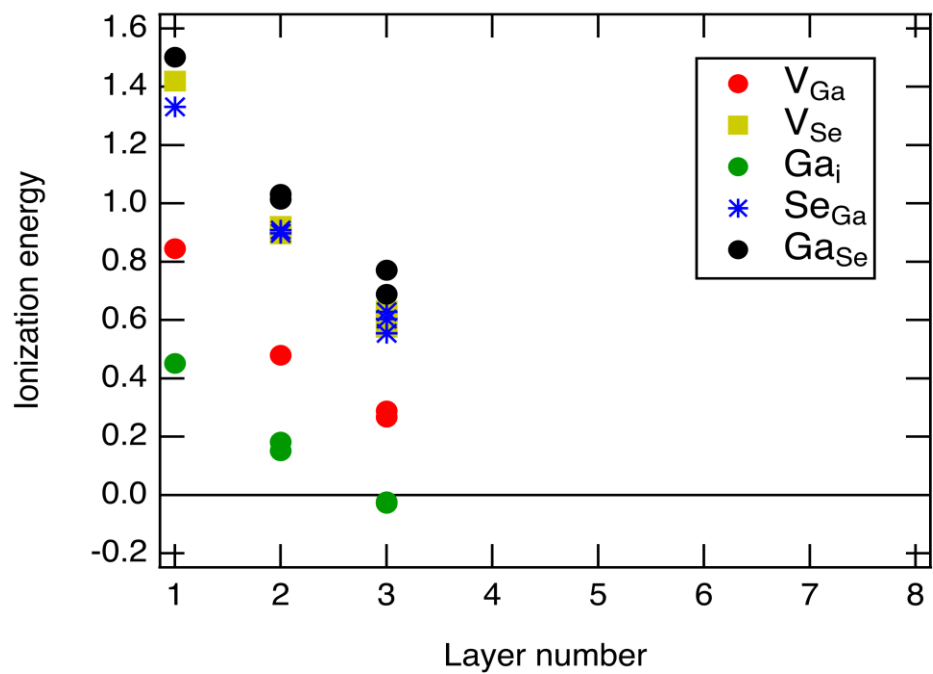

**Figure S 6:** Deviation from the bulk ionization energy of intrinsic defects as a function of layer number. Extrapolating to seven layers yields values close to zero, thus similar to the bulk.

### Formation energy of Si and O in bulk GaSe

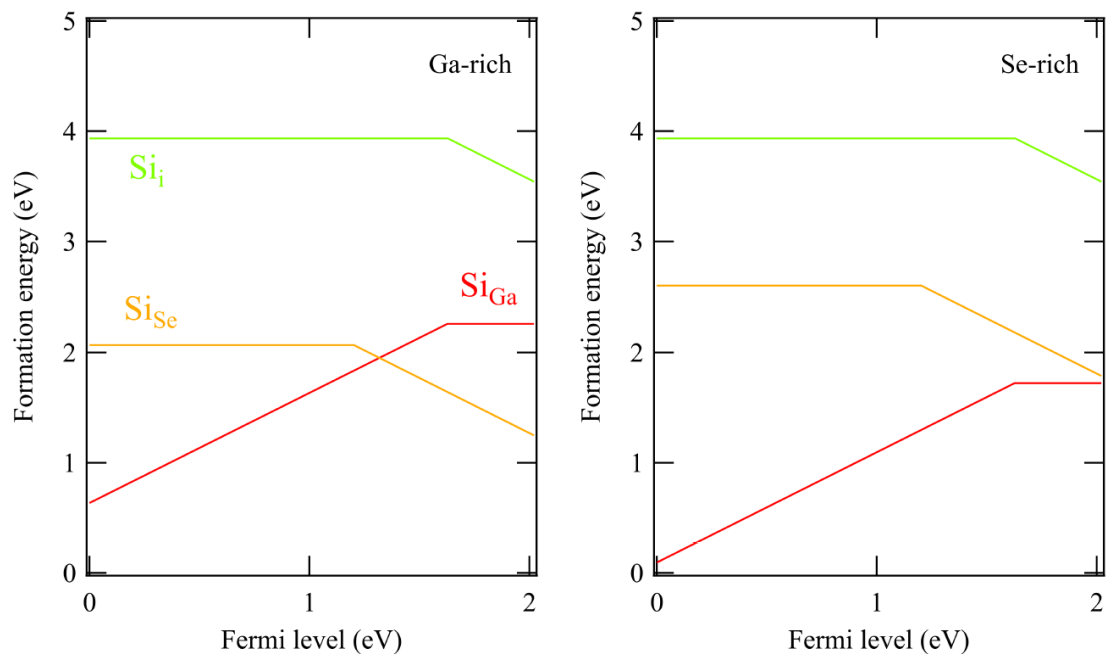

**Figure S 7:** Formation energy of Si in GaSe for Ga-rich and Se-rich conditions. The Si chemical potentials is determined by thermal equilibrium with solid Si.

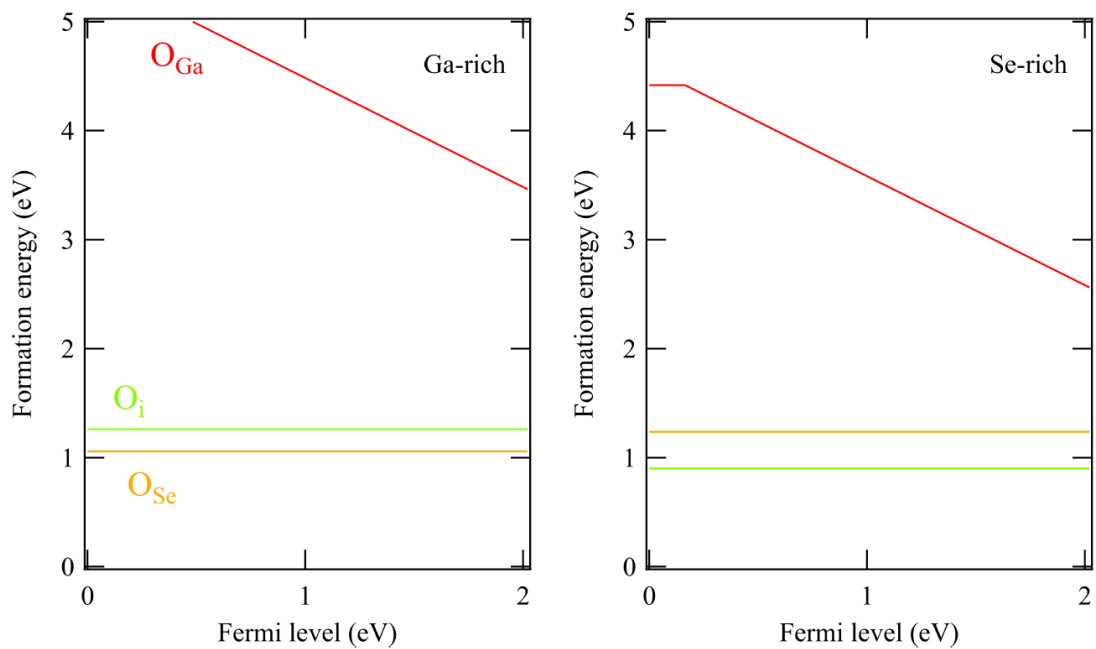

**Figure S 8:** Formation energy of O in GaSe for Ga-rich and Se-rich conditions. The O chemical potentials is determined by thermal equilibrium with solid  $\text{Ga}_2\text{O}_3$ .

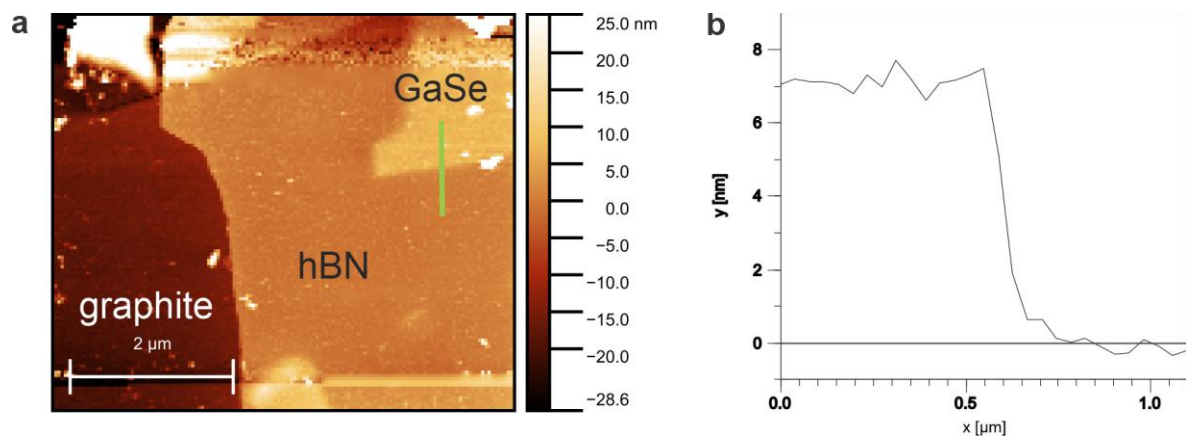

**Figure S 9:** (a) AFM scan of the GaSe MIS device. (b) Height profile along the green bar in Figure (a).
